# Supplementary material for: Artificial Neural Network Approach to the Analytic Continuation Problem
Source: arXiv:1810.00913 ancillary file (2020-02-06)
Supplement: Supplementary file 1 [file supp_mat.pdf]

# Supplemental Material for
# "Artificial Neural Network Approach to the Analytic Continuation Problem"

Romain Fournier,[1] Lei Wang,[2] Oleg V. Yazyev,[1,3,*] and QuanSheng Wu[1,3,†]

[1] *Institute of Physics, Ecole Polytechnique Fédérale de Lausanne (EPFL), CH-1015 Lausanne, Switzerland*
[2] *Institute of Physics, Chinese Academy of Sciences, Beijing 100190, China*
[3] *National Centre for Computational Design and Discovery of Novel Materials MARVEL, Ecole Polytechnique Fédérale de Lausanne (EPFL), CH-1015 Lausanne, Switzerland*

## A. Quantum Monte Carlo (QMC) simulations

In this section of the Supplemental Material document, we briefly present the derivation of the formalism used to perform the Monte Carlo sampling of the imaginary-time correlation function $c(\tau)$. Starting with the equation present in the main text

$$c(\tau) = \int_{-\infty}^{\infty} e^{-\omega(\tau-\frac{\beta}{2})} \mathrm{I}(\omega) d\omega, \tag{1}$$

we can use the Feynman-Vernon relation [1] to express the imaginary-time correlation function as

$$c\left(\tau\right) = \frac{1}{Z} \int_{x(0)=x(\beta)} D[x\left(z\right)]\, x\left(0\right) x\left(\tau\right) e^{-\beta(H[x]+S_I[x])} \tag{2}$$

with $Z$ being the partition function at inverse temperature $\beta$, $H$ the classical Hamiltonian of the system,

$$S_I\left[x\right] = -\frac{1}{2\beta} \int_0^\beta \mathrm{d}\tau \int_0^\beta \mathrm{d}\tau'\; x\left(\tau\right) L\left(\left|\tau - \tau'\right|\right) x\left(\tau'\right)$$

and

$$L(\tau) = \beta \int_0^\infty d\omega\; J_B\left(\omega\right) \omega \frac{\cosh\left(\frac{\beta\omega}{2} + \omega\tau\right)}{\sinh\left(\frac{\beta\omega}{2}\right)},$$

$\tau \in [0, \beta]$ and $J_B(\omega)$ given in the main text. Eq. 2 allows computing the imaginary-time correlation function with the standard QMC approach, using $e^{-\beta(H[x]+S_I[x])}$ as the weight function. We computed the imaginary time correlation function $c(\tau)$ by setting the parameters of the friction kernel (see main text) to $\xi_0 = 225$, $a_1 = 1.486 \times 10^5$, $a_2 = 285$, $\alpha_1 = 903$, $\alpha_2 = 75.0$ and $f = 0.2$ , and the bare oscillation frequency $\omega_0 = 20$. The imaginary time function $\hat{c}(\tau)$ was sampled on 64 slices $\tau_i \in [0, \beta]$. Each slice was computed within separate simulations to ensure their independence. The correlation function was computed from a total of $6 \times 10^6$ simulations divided into 300 blocks. The results are shown in Figure 1.

In addition to QMC simulations one needs a relation between the physical parameters and the spectral density function in order to build the database. In our case, this relation can be obtained from the generalized Langevin equation [2]. The friction kernel $\xi(t)$ is related to the power spectrum $\mathrm{I}(\omega)$ through the following relations:

$$\gamma(\omega) = \gamma'(\omega) + i\gamma''(\omega) = \frac{1}{m} \int_0^\infty dt e^{i\omega t} \xi(t), \tag{3}$$

$$I(\omega) = \frac{\omega^2 \gamma'(\omega)}{\left[\omega^2 - \tilde{\omega}^2 - \omega\gamma''(\omega)\right]^2 + \left[\omega\gamma'(\omega)\right]^2}, \tag{4}$$

with $\tilde{\omega} = \sqrt{\omega_0^2 - \frac{\xi(0)}{m}}$.

It is also interesting to assess the performance of our ANN when $c(\tau)$ contains fewer points. Figure 2 shows that the important features of the power spectrum, like the peak and the low-frequency behavior, are remarkably well reproduced even when only 16 points are available.

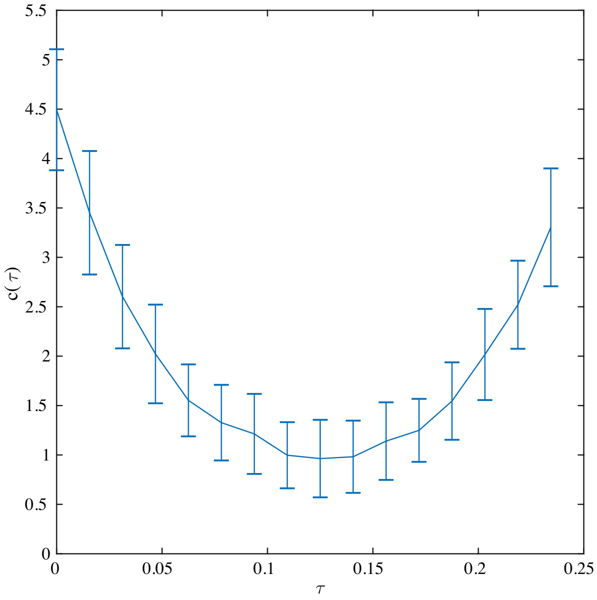


FIG. 1. Results of QMC simulations on 64 imaginary time slices with error bars representing the variance of $c(\tau)$ over 300 blocks.

* E-mail: oleg.yazyev@epfl.ch
† E-mail: quansheng.wu@epfl.ch

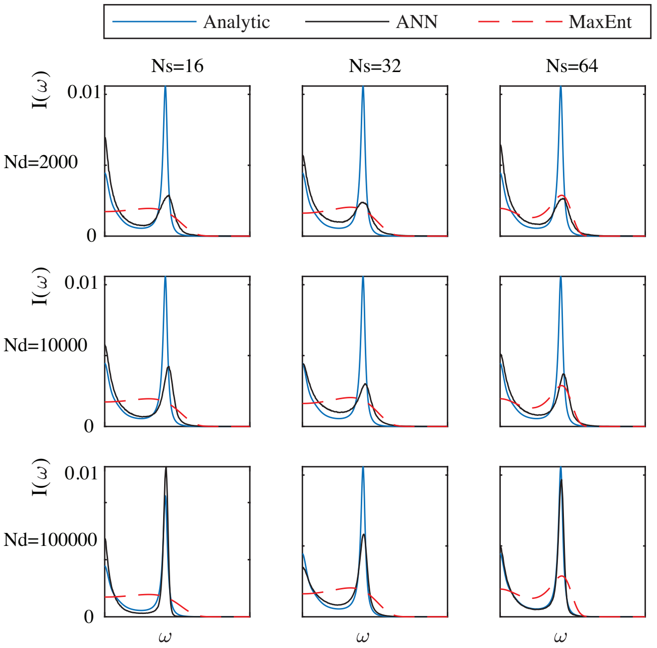


FIG. 2. Power spectra $I(\omega)$ obtained using the ANN trained on $N_d$ data entries and MaxEnt for an input data containing $N_s$ imaginary time slices in comparison with the exact solution.

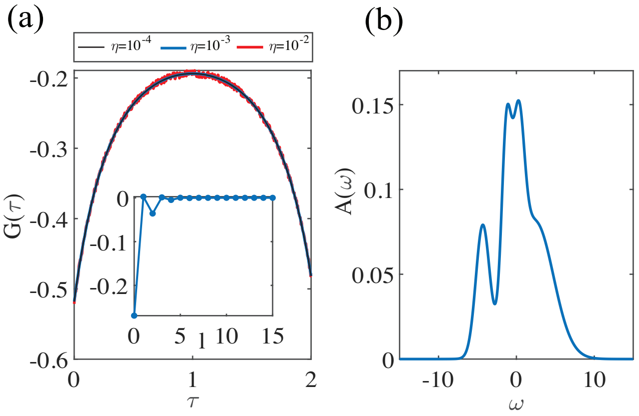


FIG. 3. (a) Example of Green's function $G(\tau)$ containing noise of three different amplitudes $\eta$ and (b) its corresponding spectral density function $A(\omega)$. The Legendre representation $G_l$ of the Green's function (without noise) is shown in panel (a) inset. Only the first 16 coefficients are displayed for clarity.

### B. Recovery of spectral density function

In order to provide direct comparison with the approach of Arsenault *et al.* [3], we generate pairs of spectral density and Green's function related by Eq. 3 of the main text. We choose to simulate spectral density functions that always has a quasiparticle peak close to $\omega = 0$ as often encountered when considering correlated metals [4, 5]. We stress that apart the final softmax layer that ensures the output to have the shape of a density function, the choice of the training data is the main source of regularization of the problem. As in Ref. [3], the model spectral densities $A(\omega)$ are defined as a sum of uncorrelated Gaussian distributions

$$A_j(\omega) = \frac{1}{N_R}\sum_{i=0}^{R_j} \exp\left(-\frac{(\omega-\mu_i)^2}{2\sigma_i^2}\right), \qquad (5)$$

where the frequencies $\omega \in [-\Omega_0, \Omega_0]$, the maximum frequency $\Omega_0 = 15$ eV, the centers of the peaks $\mu_j \in [-6, 6]$ eV, the number of Gaussian distributions $R_j \in 1, 2, ..., 21$ and their broadening $\sigma_j \in [0.1, 1]$ eV. Prefactor $1/N_R$ is used to normalize the spectrum. Parameters $R_j$, $\mu_j$ and $\sigma_j$ are uniformly sampled over the above-mentioned ranges, with the exception of $\mu_0$ that is constrained to be located close to the origin ($\mu_0 \in [-0.5, 0.5]$ eV). These spectral functions are then used to compute their corresponding Green's functions, thanks to the stability of the forward problem. A representative example of a $(G(\tau), A(\omega))$ pair is given in Fig. 3. Finding a more compact representation of the data facilitates the learning process of the model. In previous works, the orthogonal basis of Legendre polynomials was successfully used to improve results involving Green's functions [6, 7]. Applying this idea, we compute the inputs $G_l$ from $G(\tau)$ using the following definition:

$$G(\tau) = \sum_{l\geq 0}(2l+1)G_l P_l(2\frac{\tau}{\beta} - 1), \qquad (6)$$

where $P_l(x)$ are the Legendre polynomials. Fig. 3a (inset) shows that the amplitude of the coefficient associated with the Legendre polynomials decreases rapidly with increasing order.

We start designing our deep learning model by considering a fully connected 2-layer ANN trained over datasets of different sizes and test this model on a validation set composed of unseen examples (Fig. 4a). All training curves show a similar behavior. The mean absolute error (MAE) calculated on the validation dataset first decreases with increasing the number of epochs (iterations over the entire dataset) and then suddenly increases. On the other hand, MAE calculated on the training dataset decreases during the entire learning process (Fig. 4b). We conclude that our model can learns from data but starts suffering from overfitting issues after a number of epochs. Inspecting the minimum MAE reached during each training also shows that adding data is not an efficient way of achieving better accuracy (Fig. 4a, inset). Indeed, an exponentially growing number of samples is required for reducing the error linearly.

Instead, improving the training process can be achieved using common methods of deep learning, such as the batch normalization and introducing additional layers [8]. We add three dense units and normalize the data prior each of them. As seen in Fig. 4b, the training is improved, but this model fails to generalize on the validation dataset (Fig. 4c).

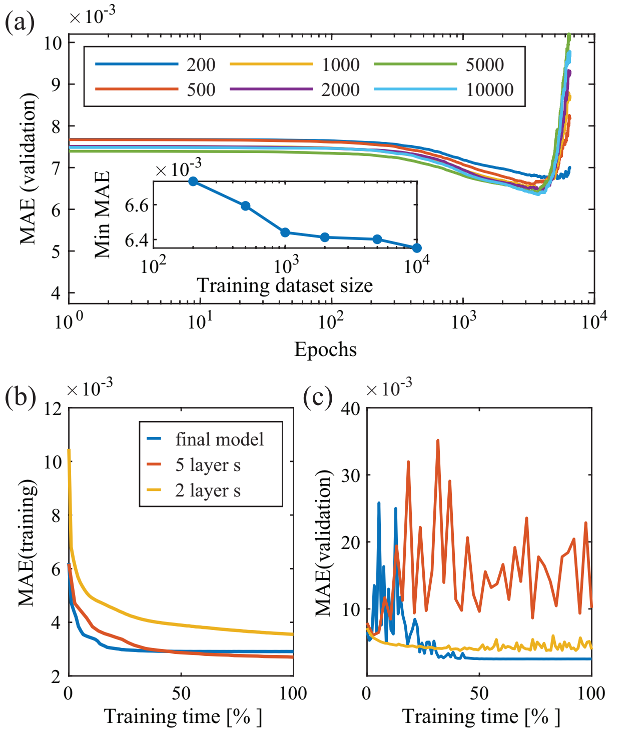


FIG. 4. (a) Training curves of a 2-layer feedfoward ANN with batch normalization. (b),(c) Comparison the training (b) and validation (c) curves of the 2-layer feedfoward ANN with batch normalization, 5-layer feedfoward ANN with batch normalization and the final model described in the main text.

We then introduce standard procedures to avoid overfitting. We reduce the learning rate, *i.e.* the speed at which the parameters are updated, when the validation score does not improve and add dropout between layers. The final architecture of our model shown in the main text consists of an input layer followed by five repetitions of a sequence of layers: a batch normalization layer to improve the training [9], a linear rectifier unit to add non-linearities into the model, a dropout unit to avoid overfitting [10] and a dense layer for the learning. Each of these layers contains 1024 units. A softmax layer plays the role of the output layer.

We test the generalization power of our model by applying it to unseen data. Fig. 5 shows that MAE remains similar to the one of the validation set, with no major changes when testing the model on bigger test sets. This implies that our model generalizes well.

We have also investigated two approaches to improving the robustness of our results against noisy input data. The first approach relies on preprocessing data using unsupervised learning. Inspired by denoising algorithms in image recognition, we adopted the principal component analysis (PCA) approach for this purpose [11, 12]. As a first step, we compute the principal components of the Legendre coefficients present in our database to form a new basis whose vectors are aligned along the direction of maximum variance in the dataset. The noisy samples

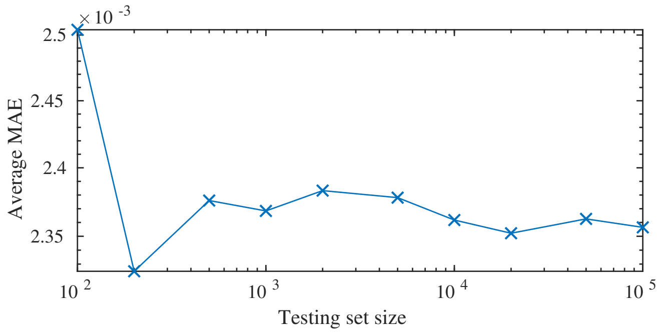


FIG. 5. The final ANN model was used on different testing sets containing an increasing number of data entries. The average MAE converges toward a solution. The result remains relatively stable for test set sizes larger than 500 entries, which was the test set size used during the training.

are then expressed in this basis, and all but the first $n$ components are set to zero. In our case, $n = 3$ components are retained, which corresponds to directions covering 99.8% of the variance of the training dataset. The data is then transformed back to the original space. This filtering approach keeps the important features of the sample while reducing the noise it contains. Examples of the filtered data are shown in Fig. 6. The second method of improving the robustness of the results only works for ANN and consists in adding a gaussian noise layer at the beginning of the network during the training phase. This layer adds random gaussian noise to the input data. Networks trained using this extra layer typically achieve better results than MaxEnt for levels of noise larger than $\eta = 10^{-4}$ by learning only from 25000 input data realizations.

Figure 7 provides a qualitative comparison of the results of our ANN model and the MaxEnt implementation of Levy *et al.* [13] for three different noise levels, $\eta = 10^{-5}$, $10^{-3}$ and $10^{-1}$, generated following the procedure described above. The level of noise was provided as parameter for MaxEnt and used to select the network for the ANN model, as explained above. In these examples, both methods predict $A(\omega)$ accurately for the lowest level of noise. However, at $\eta = 10^{-3}$ MaxEnt tends to miss peaks in the predicted spectral function $\hat{A}(\omega)$, while in the case of ANN this tendency is much less pronounced. At the highest level of noise $\eta = 10^{-1}$, our ANN model is able to correctly identify most peaks, whereas MaxEnt flattens the spectrum completely (Fig. 8). We have also compared our ANN model with the on an example from Ref. 13 used for demonstrating the capabilities of the MaxEnt method. Fig. 9 clearly shows that our ANN model is more accurate.

One drawback of our approach is that a particular inverse temperature $\beta = 2$ is imposed. It is therefore interesting to analyze in detail the effect changing temperature on the performance of the proposed ANN model. Fig. 10 shows that compared to optimal $\beta = 2$ larger inverse temperatures tend to broaden the peaks and dis-

place the spectral weight towards higher frequencies. The opposite is true for smaller inverse temperatures. The peaks are sharper and closer to the center. In this range of temperatures, however, the shapes of the peaks remain consistent. Therefore, we conclude that our model is stable against small variation of temperature.


[1] R. Feynman and F. Vernon, Annals of Physics **281**, 547 (2000).

[2] B. J. Berne, M. E. Tuckerman, J. E. Straub, and A. L. R. Bug, J. Chem. Phys. **93**, 5084 (1990).

[3] L.-F. Arsenault, R. Neuberg, L. A. Hannah, and A. J. Millis, Inverse Problems **33**, 115007 (2017).

[4] F. Zhang and T. Rice, Physical Review B **37**, 3759 (1988).

[5] J. Kondo, Progress of theoretical physics **32**, 37 (1964).

[6] L. Huang, Chin. Phys. B **25**, 117101 (2016).

[7] Q.-S. Wu, Y.-L. Wang, Z. Fang, and X. Dai, Chin. Phys. Lett. **30**, 090201 (2013).

[8] I. Goodfellow, Y. Bengio, and A. Courville, *Deep Learning* (MIT Press, 2016).

[9] S. Ioffe and C. Szegedy, in *ICML* (2015).

[10] N. Srivastava, G. Hinton, A. Krizhevsky, I. Sutskever, and R. Salakhutdinov, Journal of Machine Learning Research **15**, 1929 (2014).

[11] I. T. Jolliffe, *Principal Component Analysis*, 2nd ed., Springer Series in Statistics (Springer-Verlag, New York, 2002).

[12] L. Zhang, W. Dong, D. Zhang, and G. Shi, Pattern Recognition **43**, 1531 (2010).

[13] R. Levy, J. LeBlanc, and E. Gull, Computer Physics Communications **215**, 149 (2017).

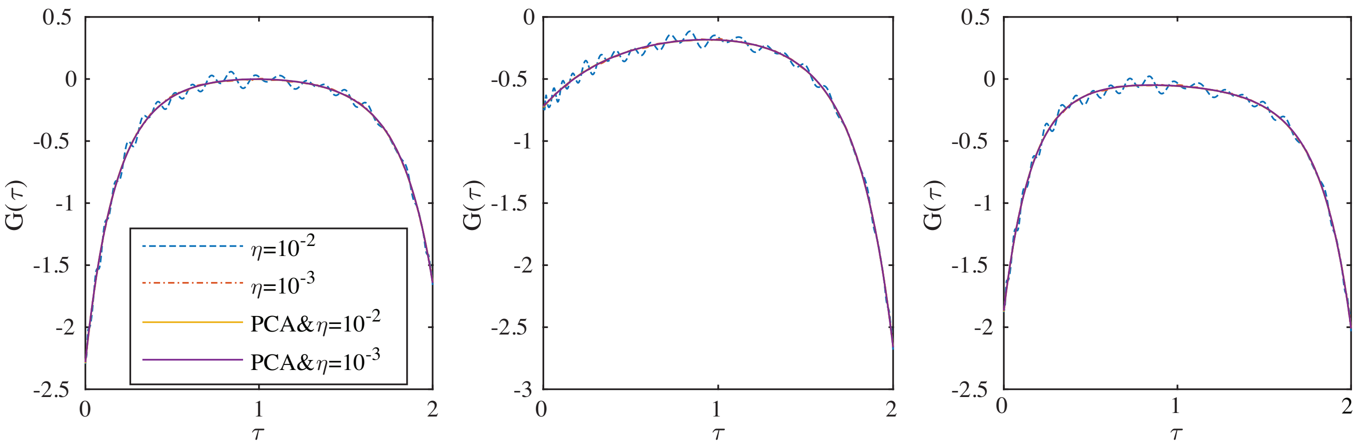


FIG. 6. Three different Green's functions at two different levels of noise $\eta$. The oscillations are not visible following the PCA filtering.

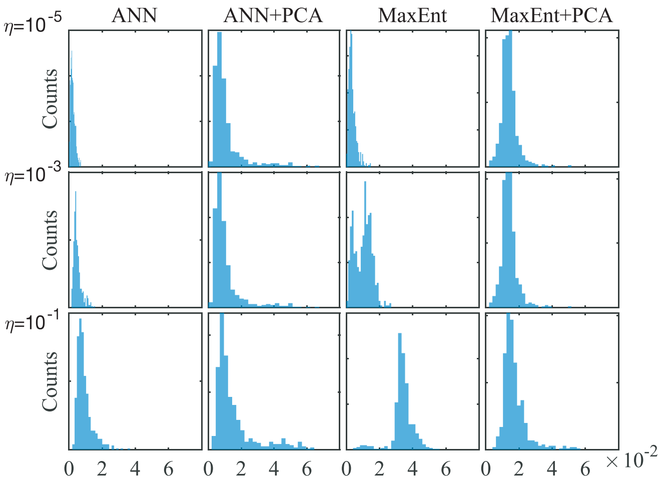


FIG. 7. MAE distributions for the ANN model and the MaxEnt method, with and without the PCA step, and at different levels of noise $\eta$. Adding a PCA step makes the model more robust with respect to noise.

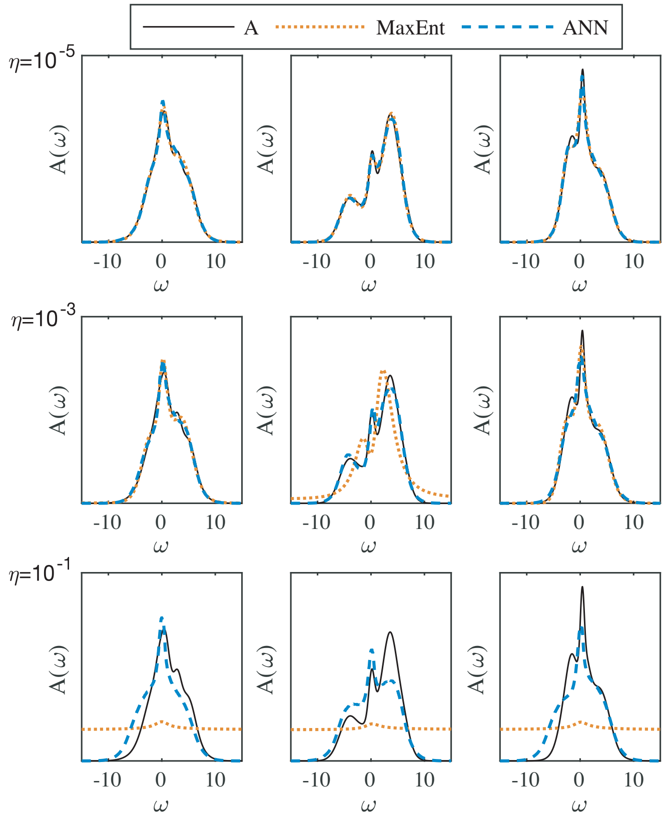


FIG. 8. Comparison of the starting spectral functions $A(\omega)$ (solid lines) with the predicted $\hat{A}(\omega)$ calculated using the MaxEnt approach and the proposed ANN model (dashed lines). Different noise levels $\eta$ are applied to the Green's functions of the three examples of spectral density functions.

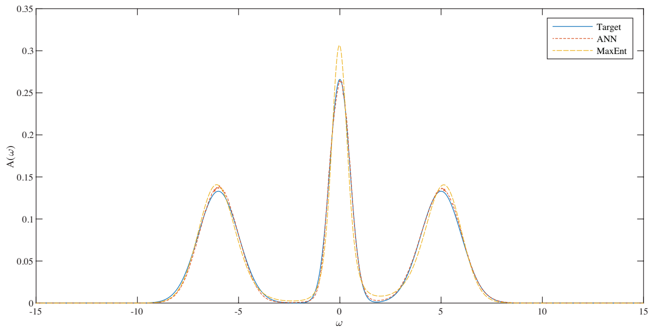


FIG. 9. Comparison of the proposed ANN model performance with that of the MaxEnt example from Ref. 13. The target spectral density function is the reference exact result.

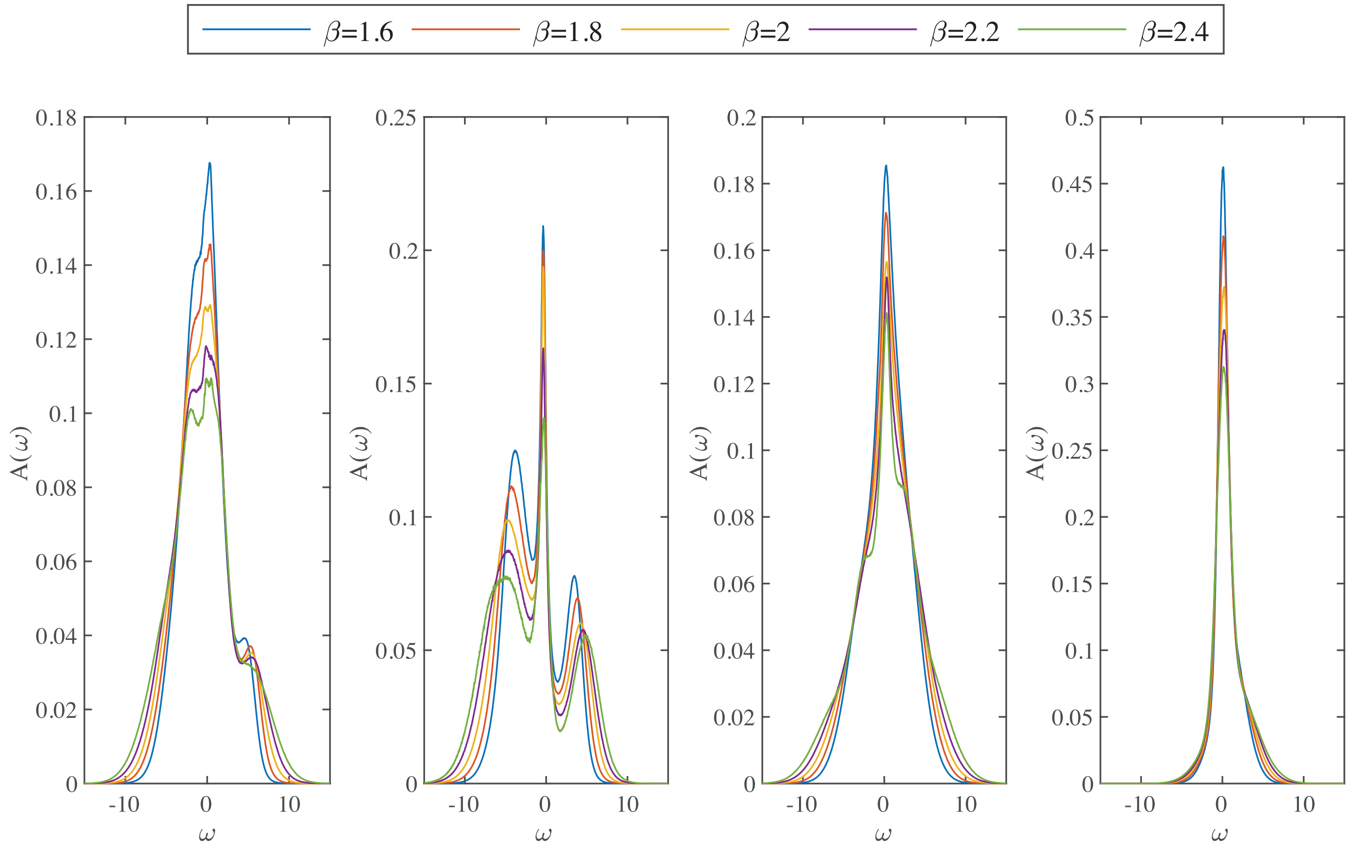


FIG. 10. Predicted spectral density functions $A(\omega)$ for four representative Green's functions $G(\tau)$ at different values of inverse temperature $\beta$.
